# Supplementary material for: Building a Subspace of Policies for Scalable Continual Learning
Source: arXiv:2211.10445 source file (2023-03-02)
Supplement: Supplementary file 3 [file OLD_broader_impact_statement.tex]

\section{Broader Impact Statement}
\label{app:broader}

This work proposes a new method for the continual reinforcement learning setting, which is a very broad framework. Many real-world applications can be framed as continual RL problems. For example, household robots need to constantly learn new skills and adapt to their changing environments. Similarly, online recommendation systems need to adapt to each user and their changing preferences. Like other continual RL algorithms, our method aims to learn a policy which maximizes reward on a sequence of tasks (each of them with a corresponding reward function). The tasks or reward functions are typically specified by the designer. Depending on the goals of the designer, executing the resulting policy could result in positive or negative consequences.
