# Supplementary material for: Building a Subspace of Policies for Scalable Continual Learning
Source: arXiv:2211.10445 source file (2023-03-02)
Supplement: Supplementary file 4 [file OLD_compute_resources.tex]

\section{Compute Resources}
\label{app:compute}
Each algorithm was trained using two Intel(R) Xeon(R) CPU cores (E5-2698 v4 @ 2.20GHz) and one NVIDIA GP100 GPU. We used PyTorch \cite{pytorch} for all our experiments. Each run took between approximately 8 and 30 hours to complete. The total runtime depended on three factors: the computation time of the algorithm, the length of the scenario, and the behavior of the policy. 

The paper includes a total of xx experiments, over 10 different CRL scenarios with 46 different RL environments. Each experiment takes on average 15 hours on 1 GPU (NVIDIA V100). The means and standard deviations are computed over 10 runs unless otherwise noted.~\todo{}
