# Supplementary material for: Building a Subspace of Policies for Scalable Continual Learning
Source: arXiv:2211.10445 source file (2023-03-02)
Supplement: Supplementary file 5 [file OLD_detailed_results.tex]

\section{Detailed Results}
\label{app:results}

\begin{figure}[!]
     \adjustbox{center}{
     \begin{subfigure}[b]{0.4\textwidth}
        \includegraphics[width=\textwidth]{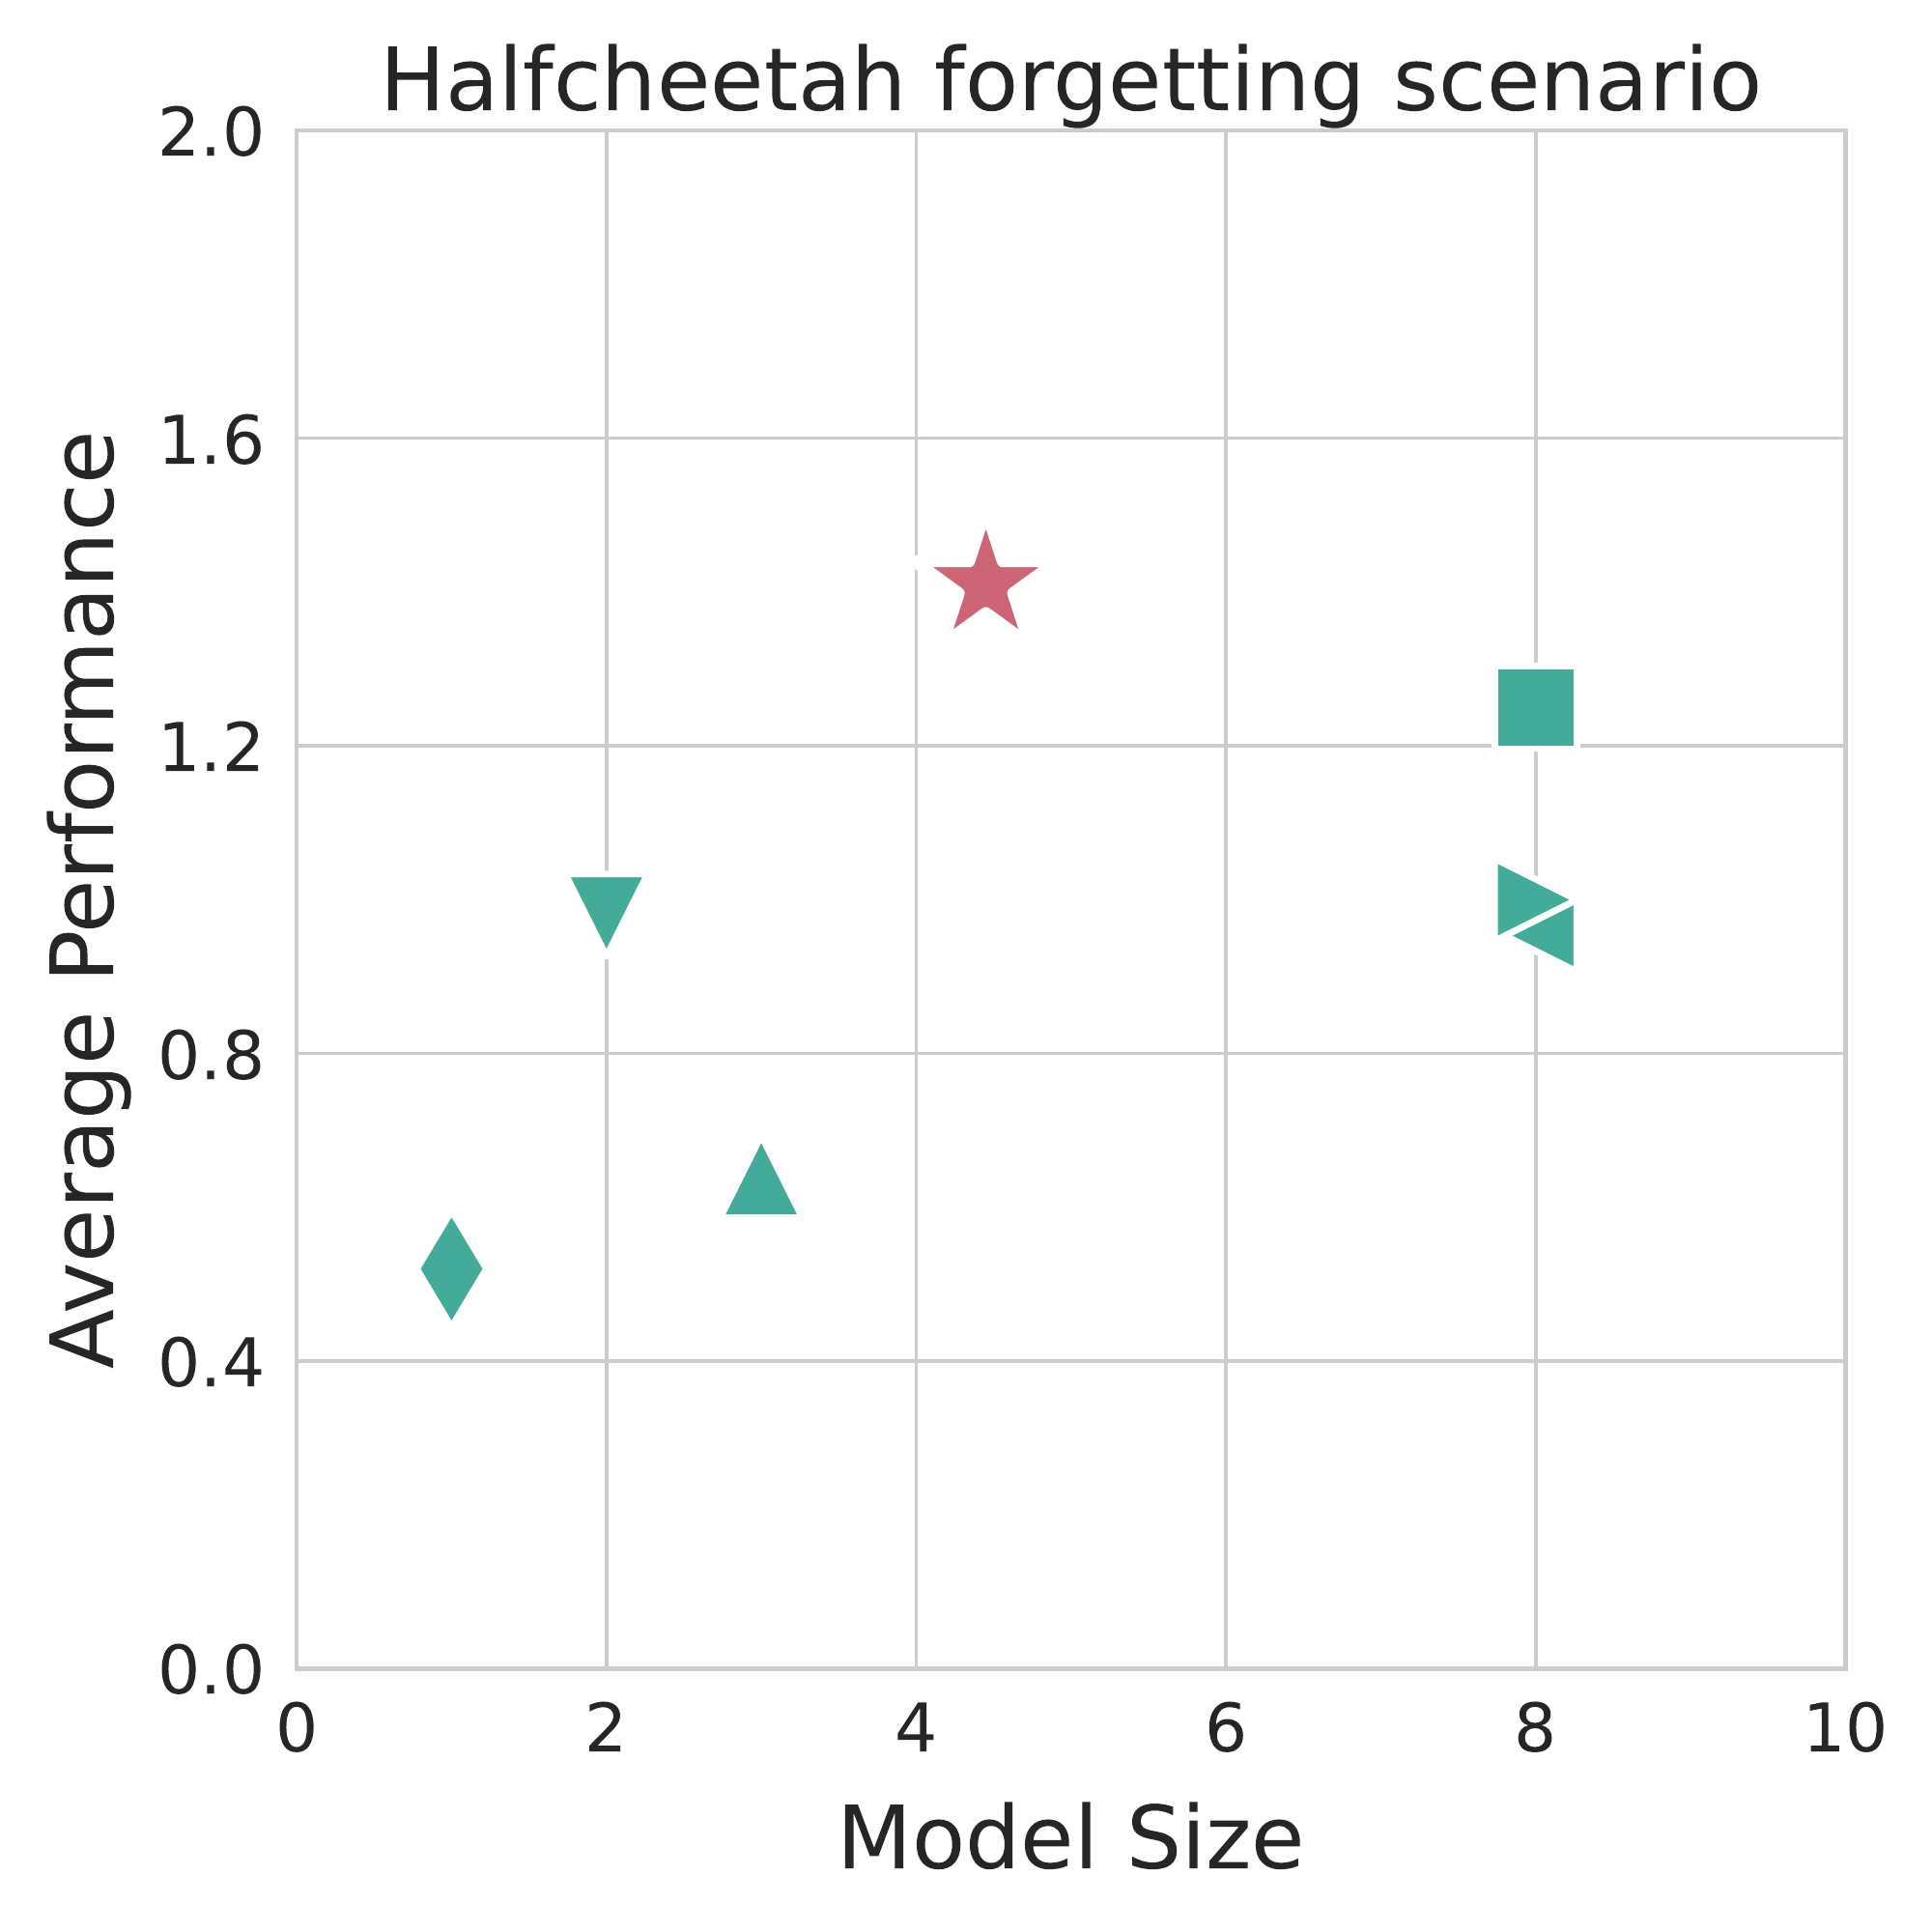}
     \end{subfigure}
     \hfill
     \begin{subfigure}[b]{0.4\textwidth}
        \includegraphics[width=\textwidth]{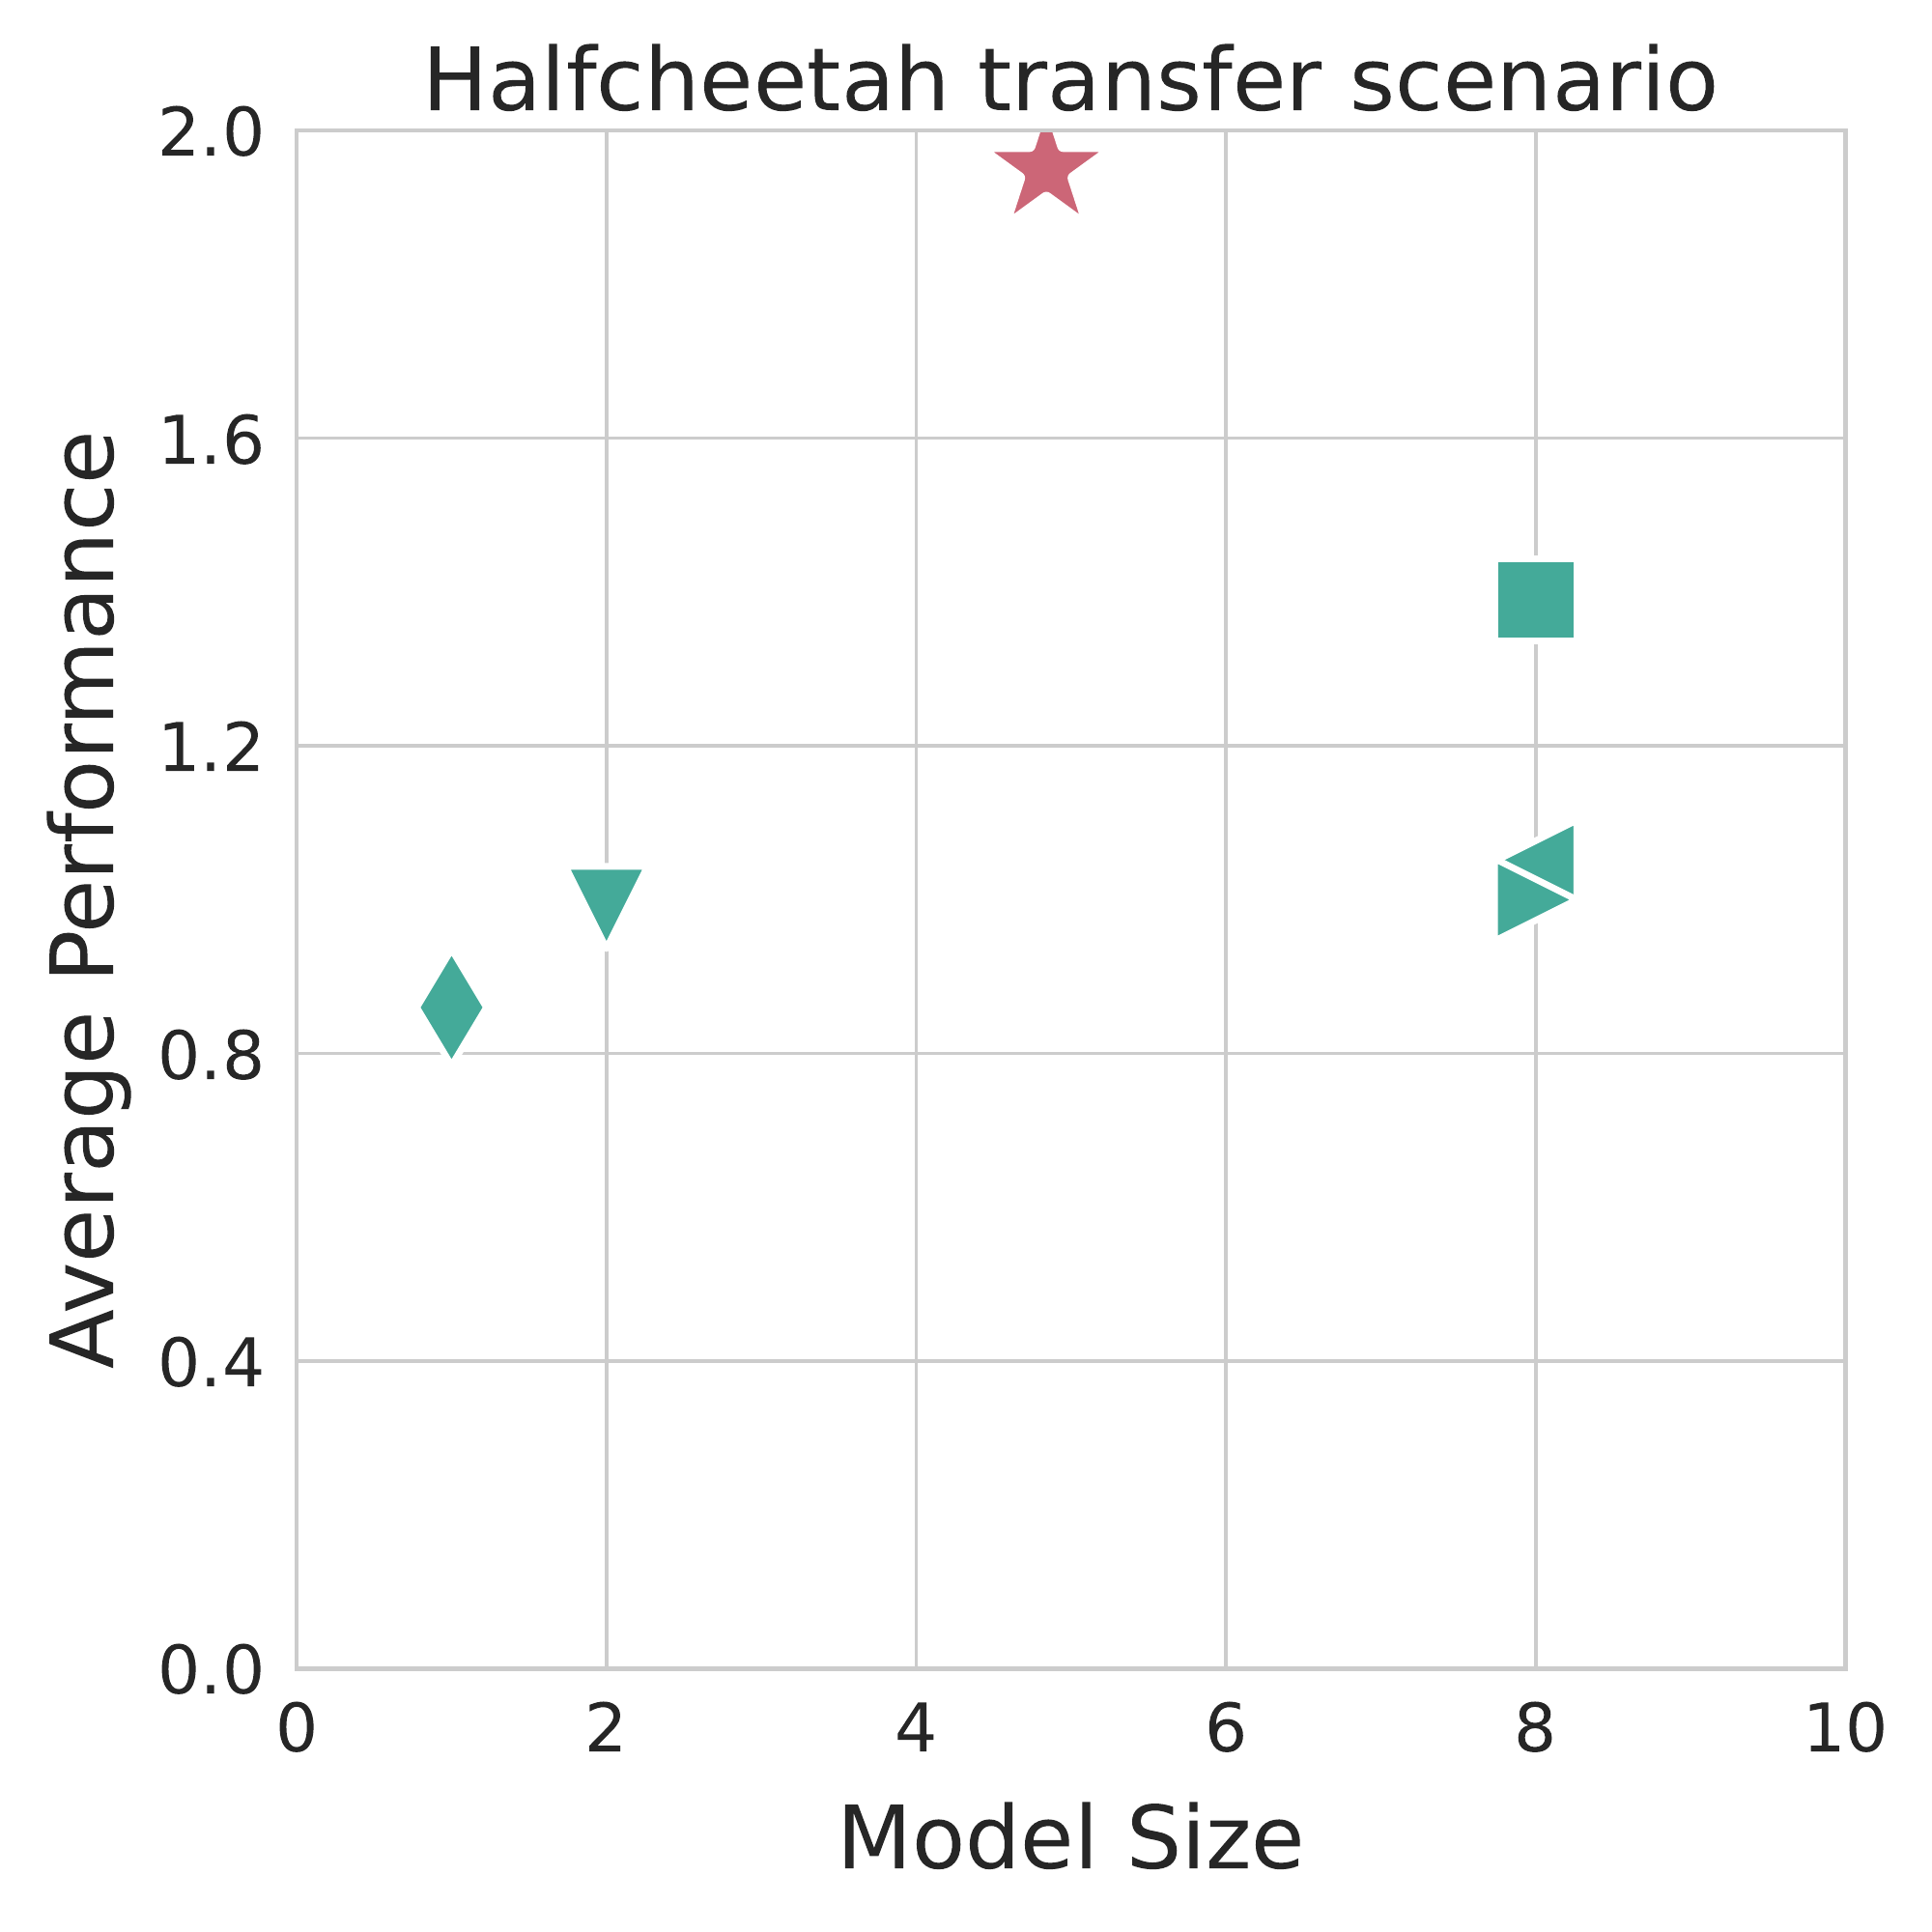}
     \end{subfigure}
     \hfill
     \begin{subfigure}[b]{0.4\textwidth}
        \includegraphics[width=\textwidth]{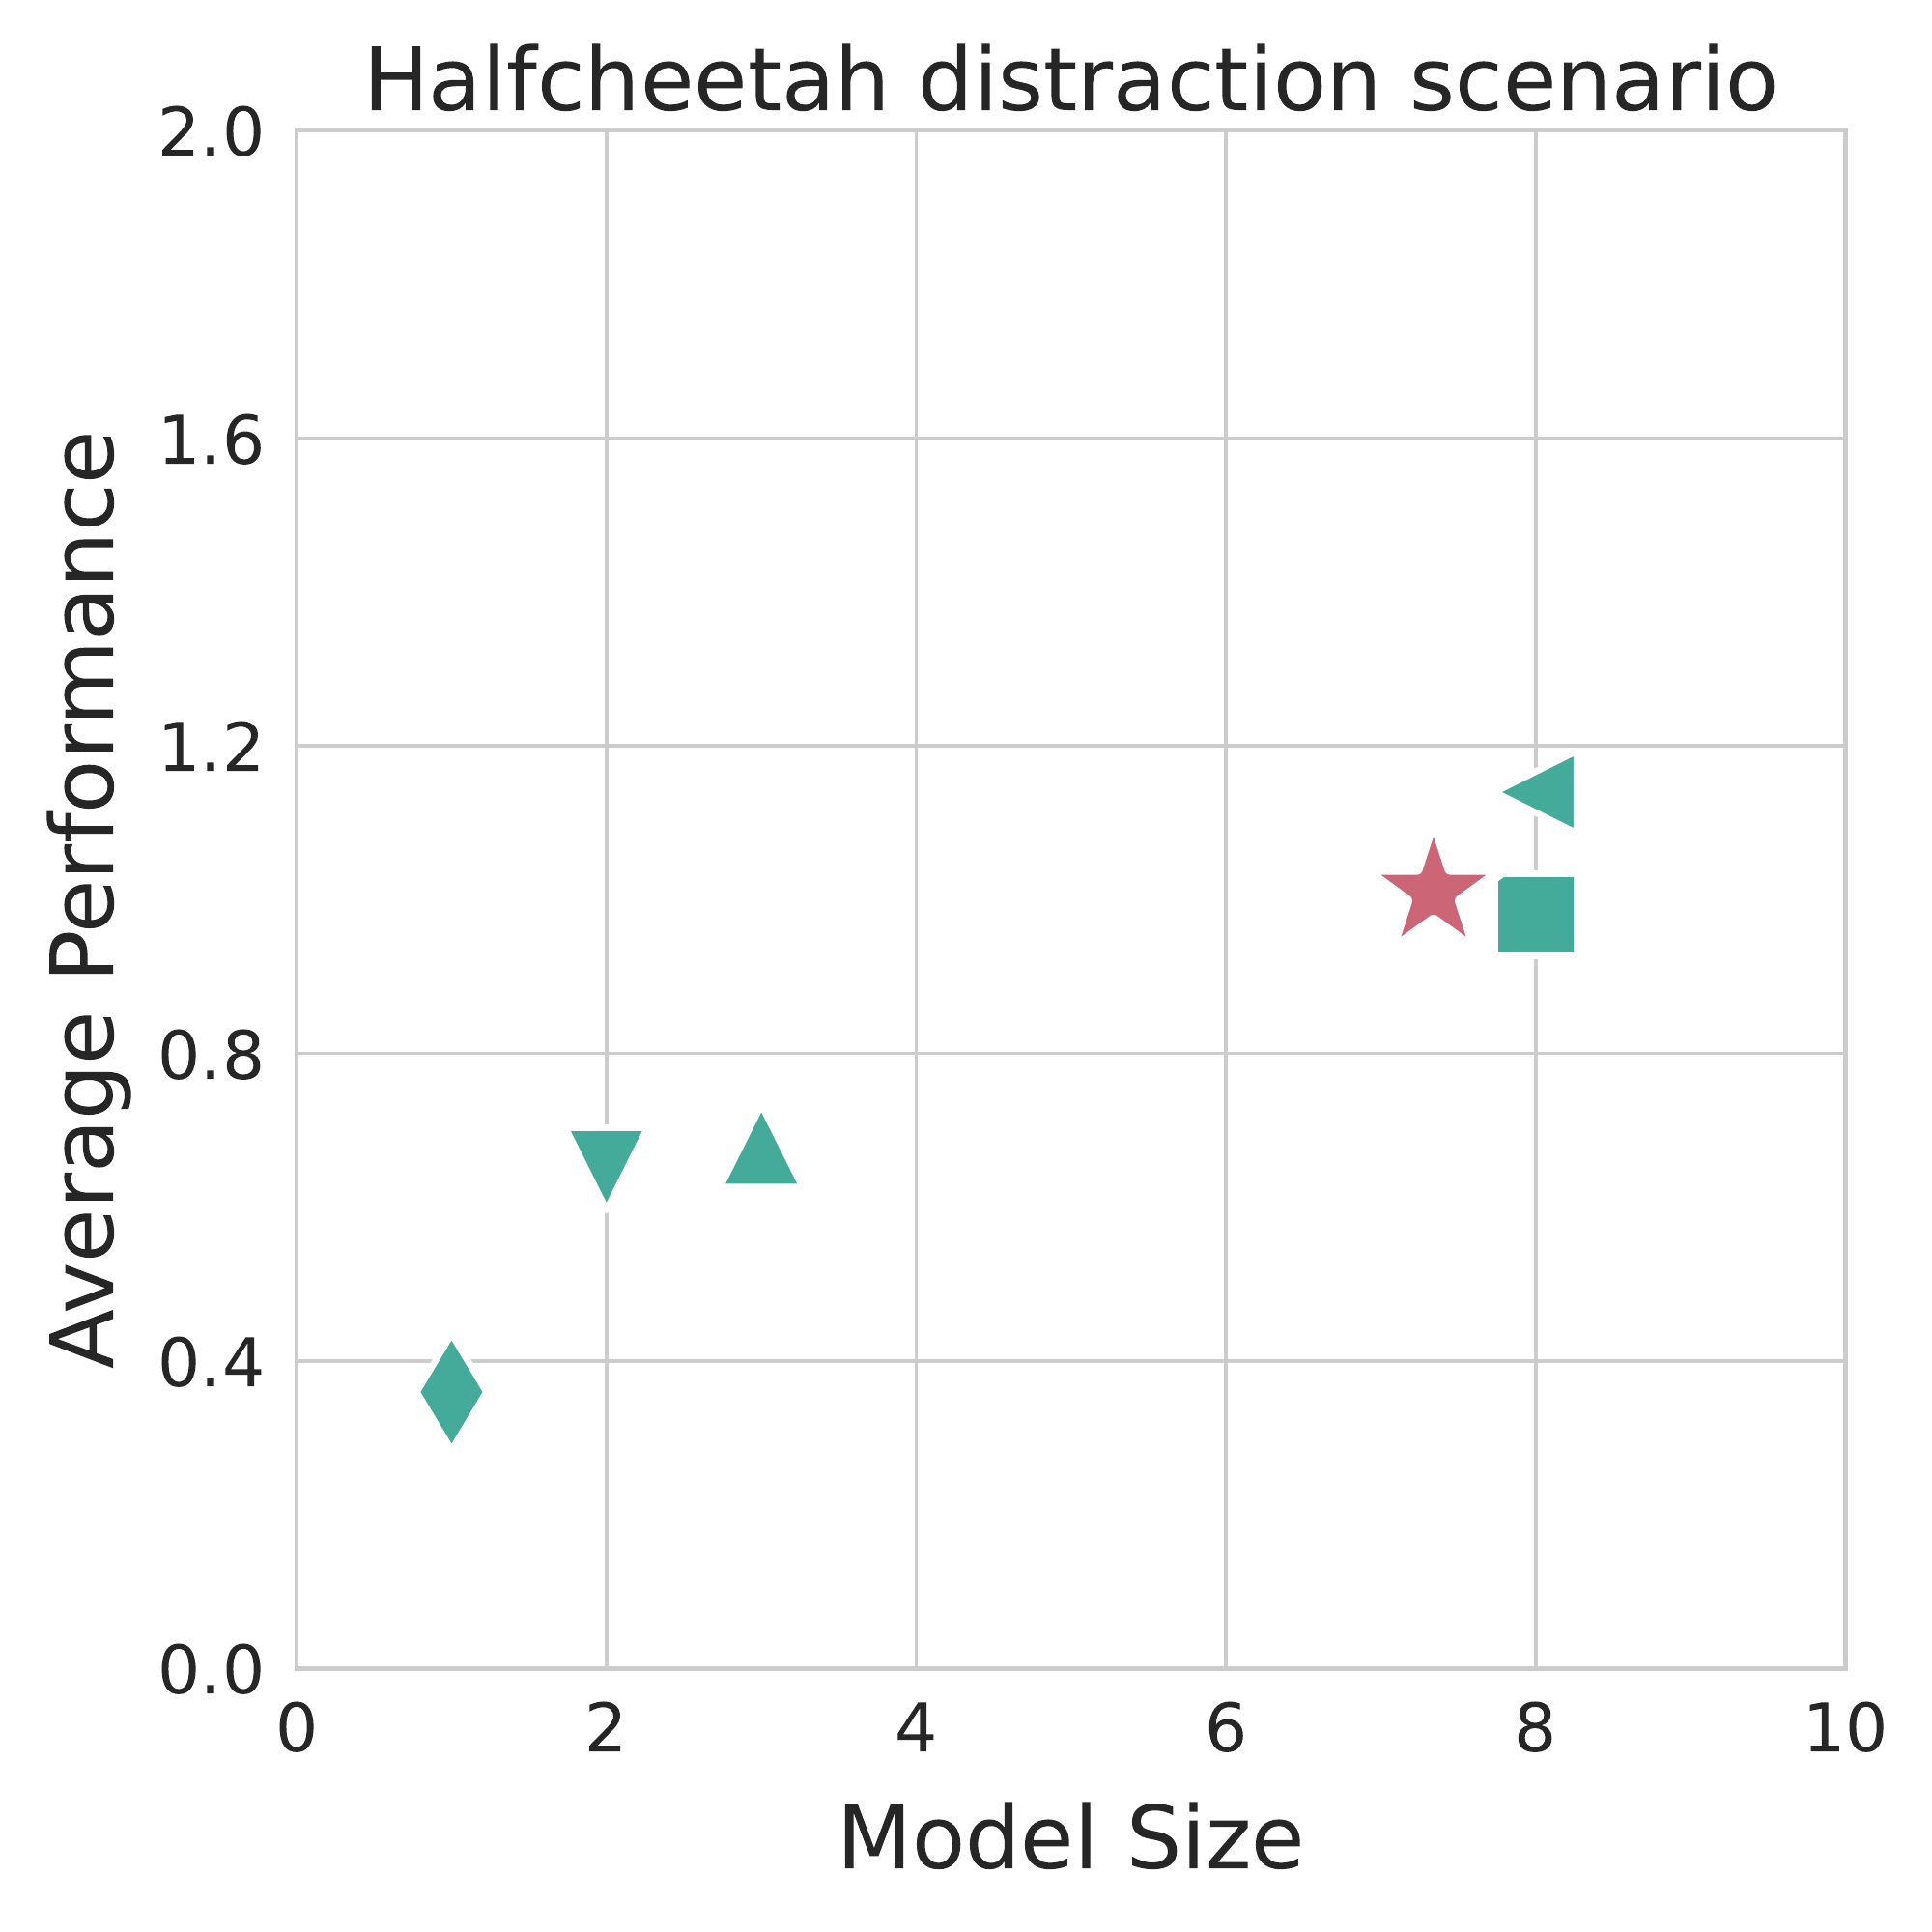}
     \end{subfigure}}
     \\
     \adjustbox{center}{
     \begin{subfigure}[b]{0.4\textwidth}

        \includegraphics[width=\textwidth]{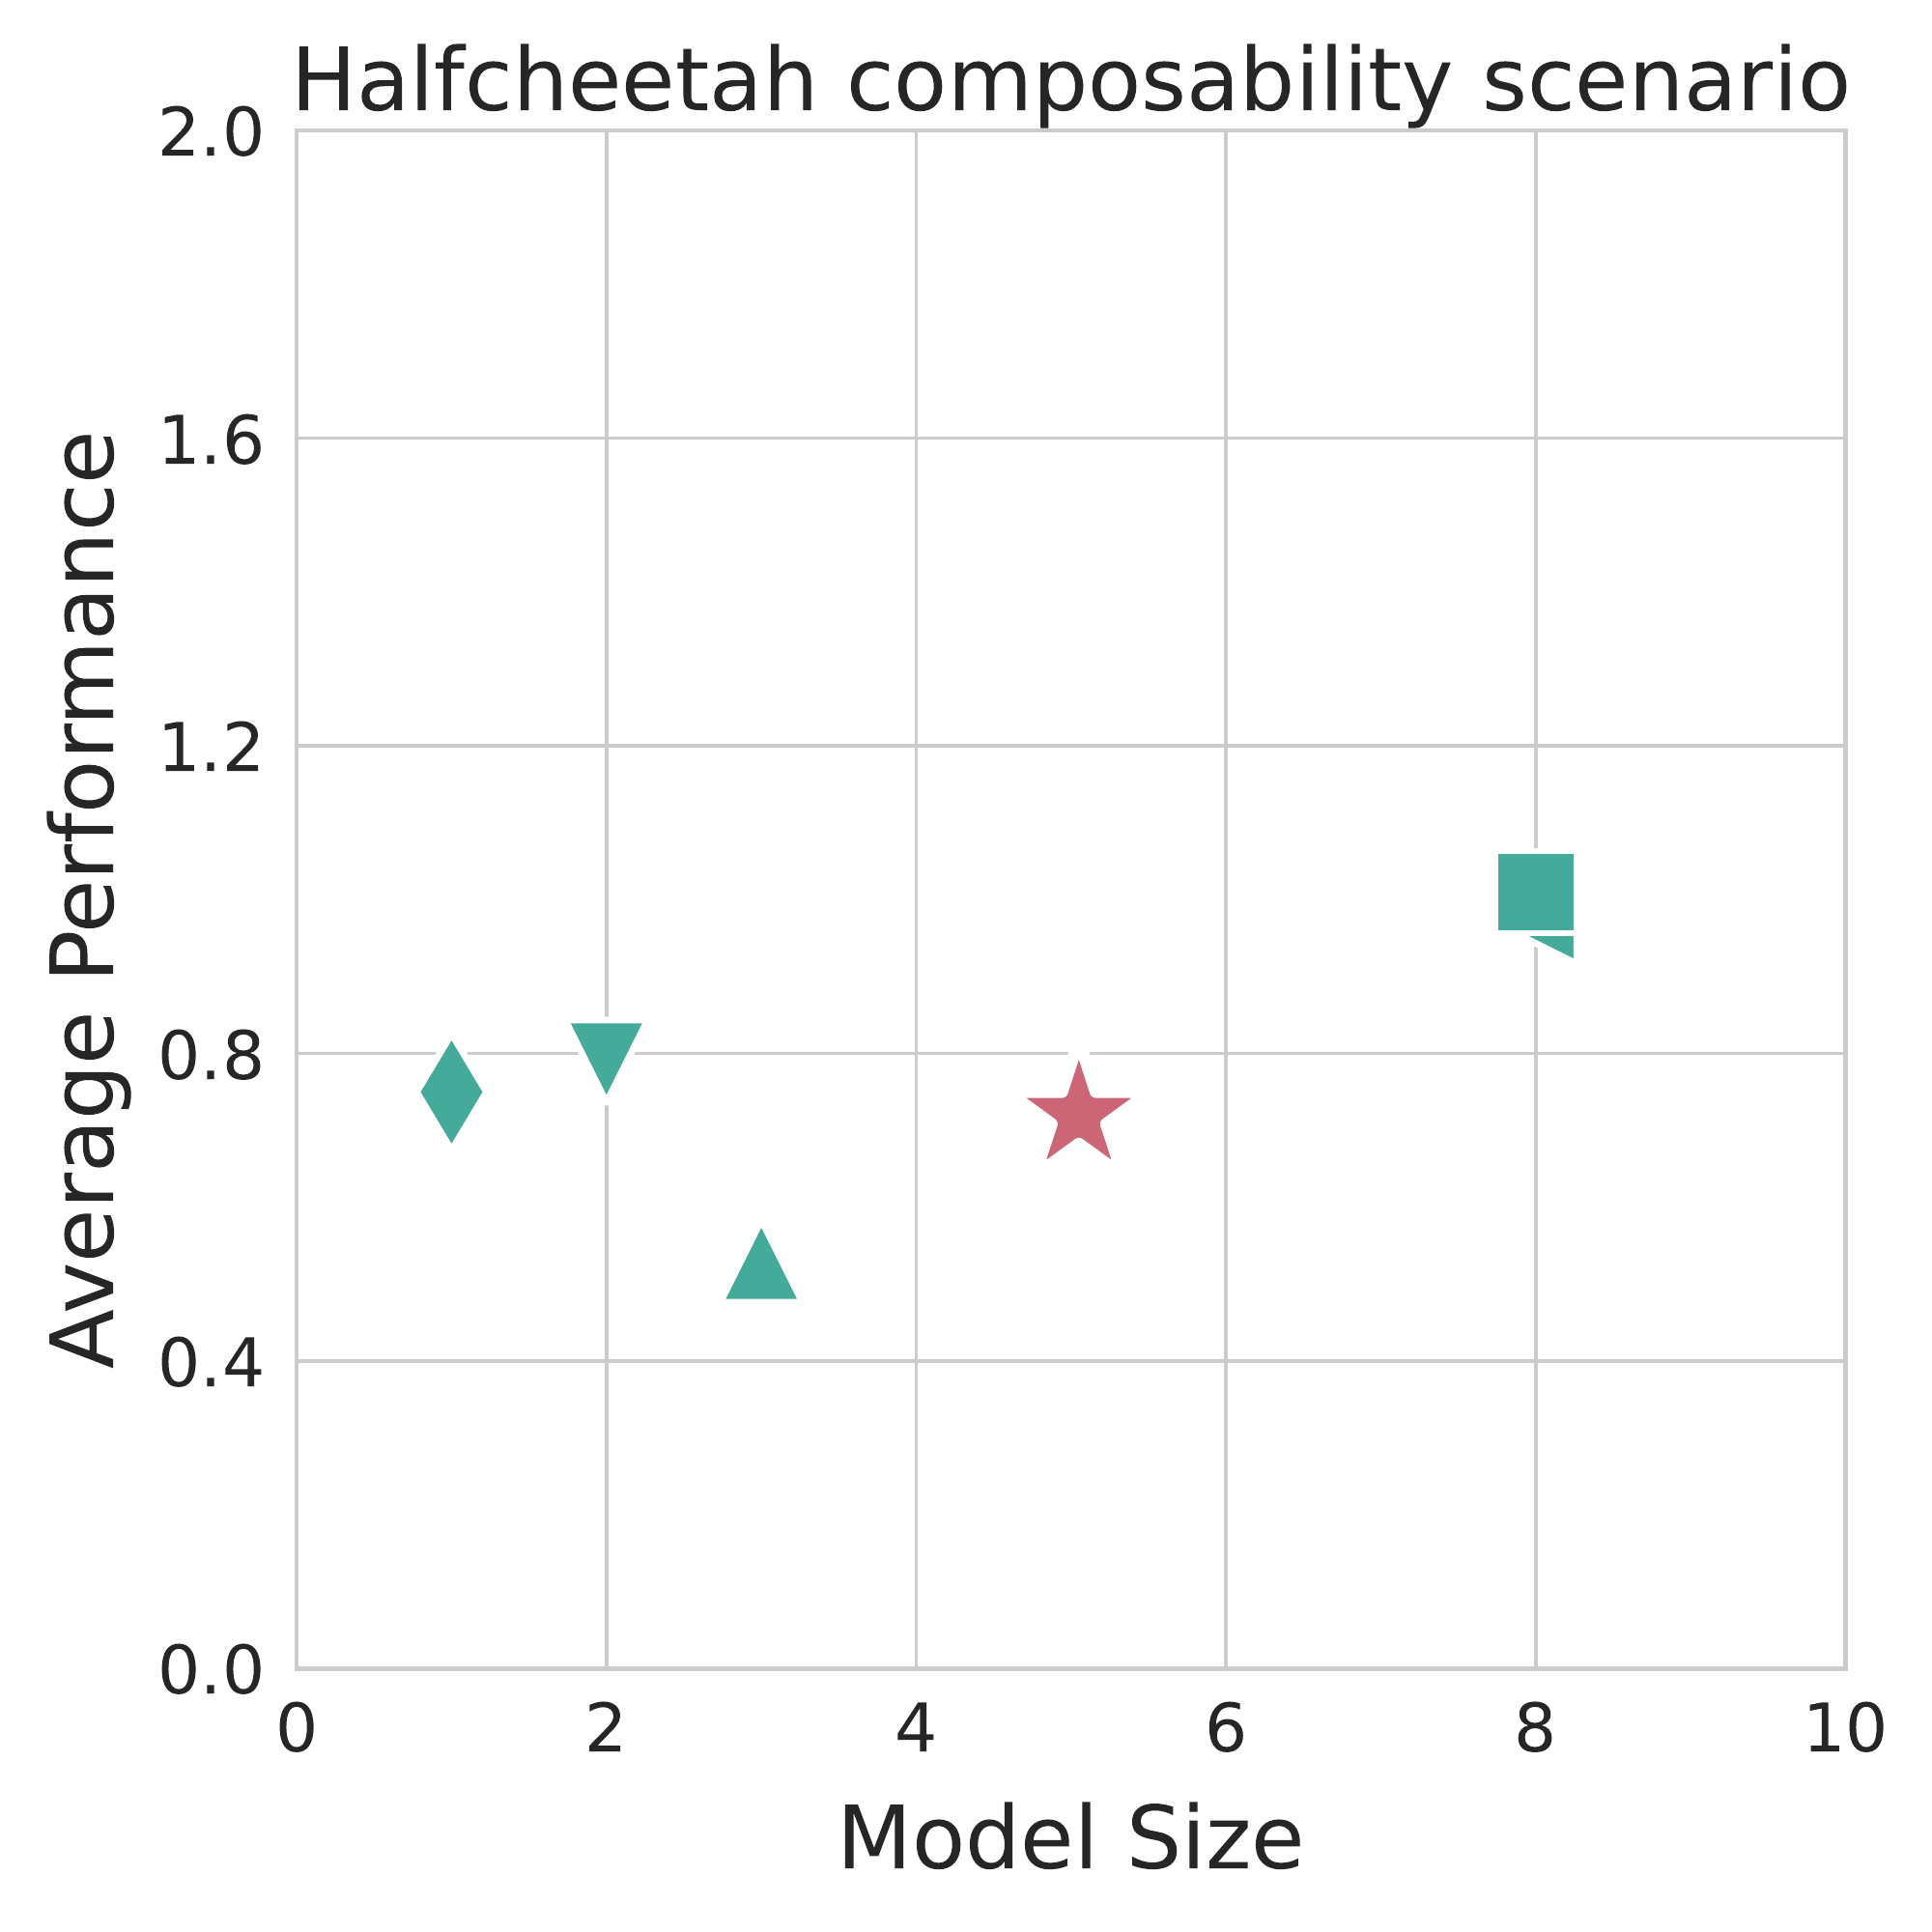}
     \end{subfigure}
     \hfill
     \begin{subfigure}[b]{0.4\textwidth}

        \includegraphics[width=\textwidth]{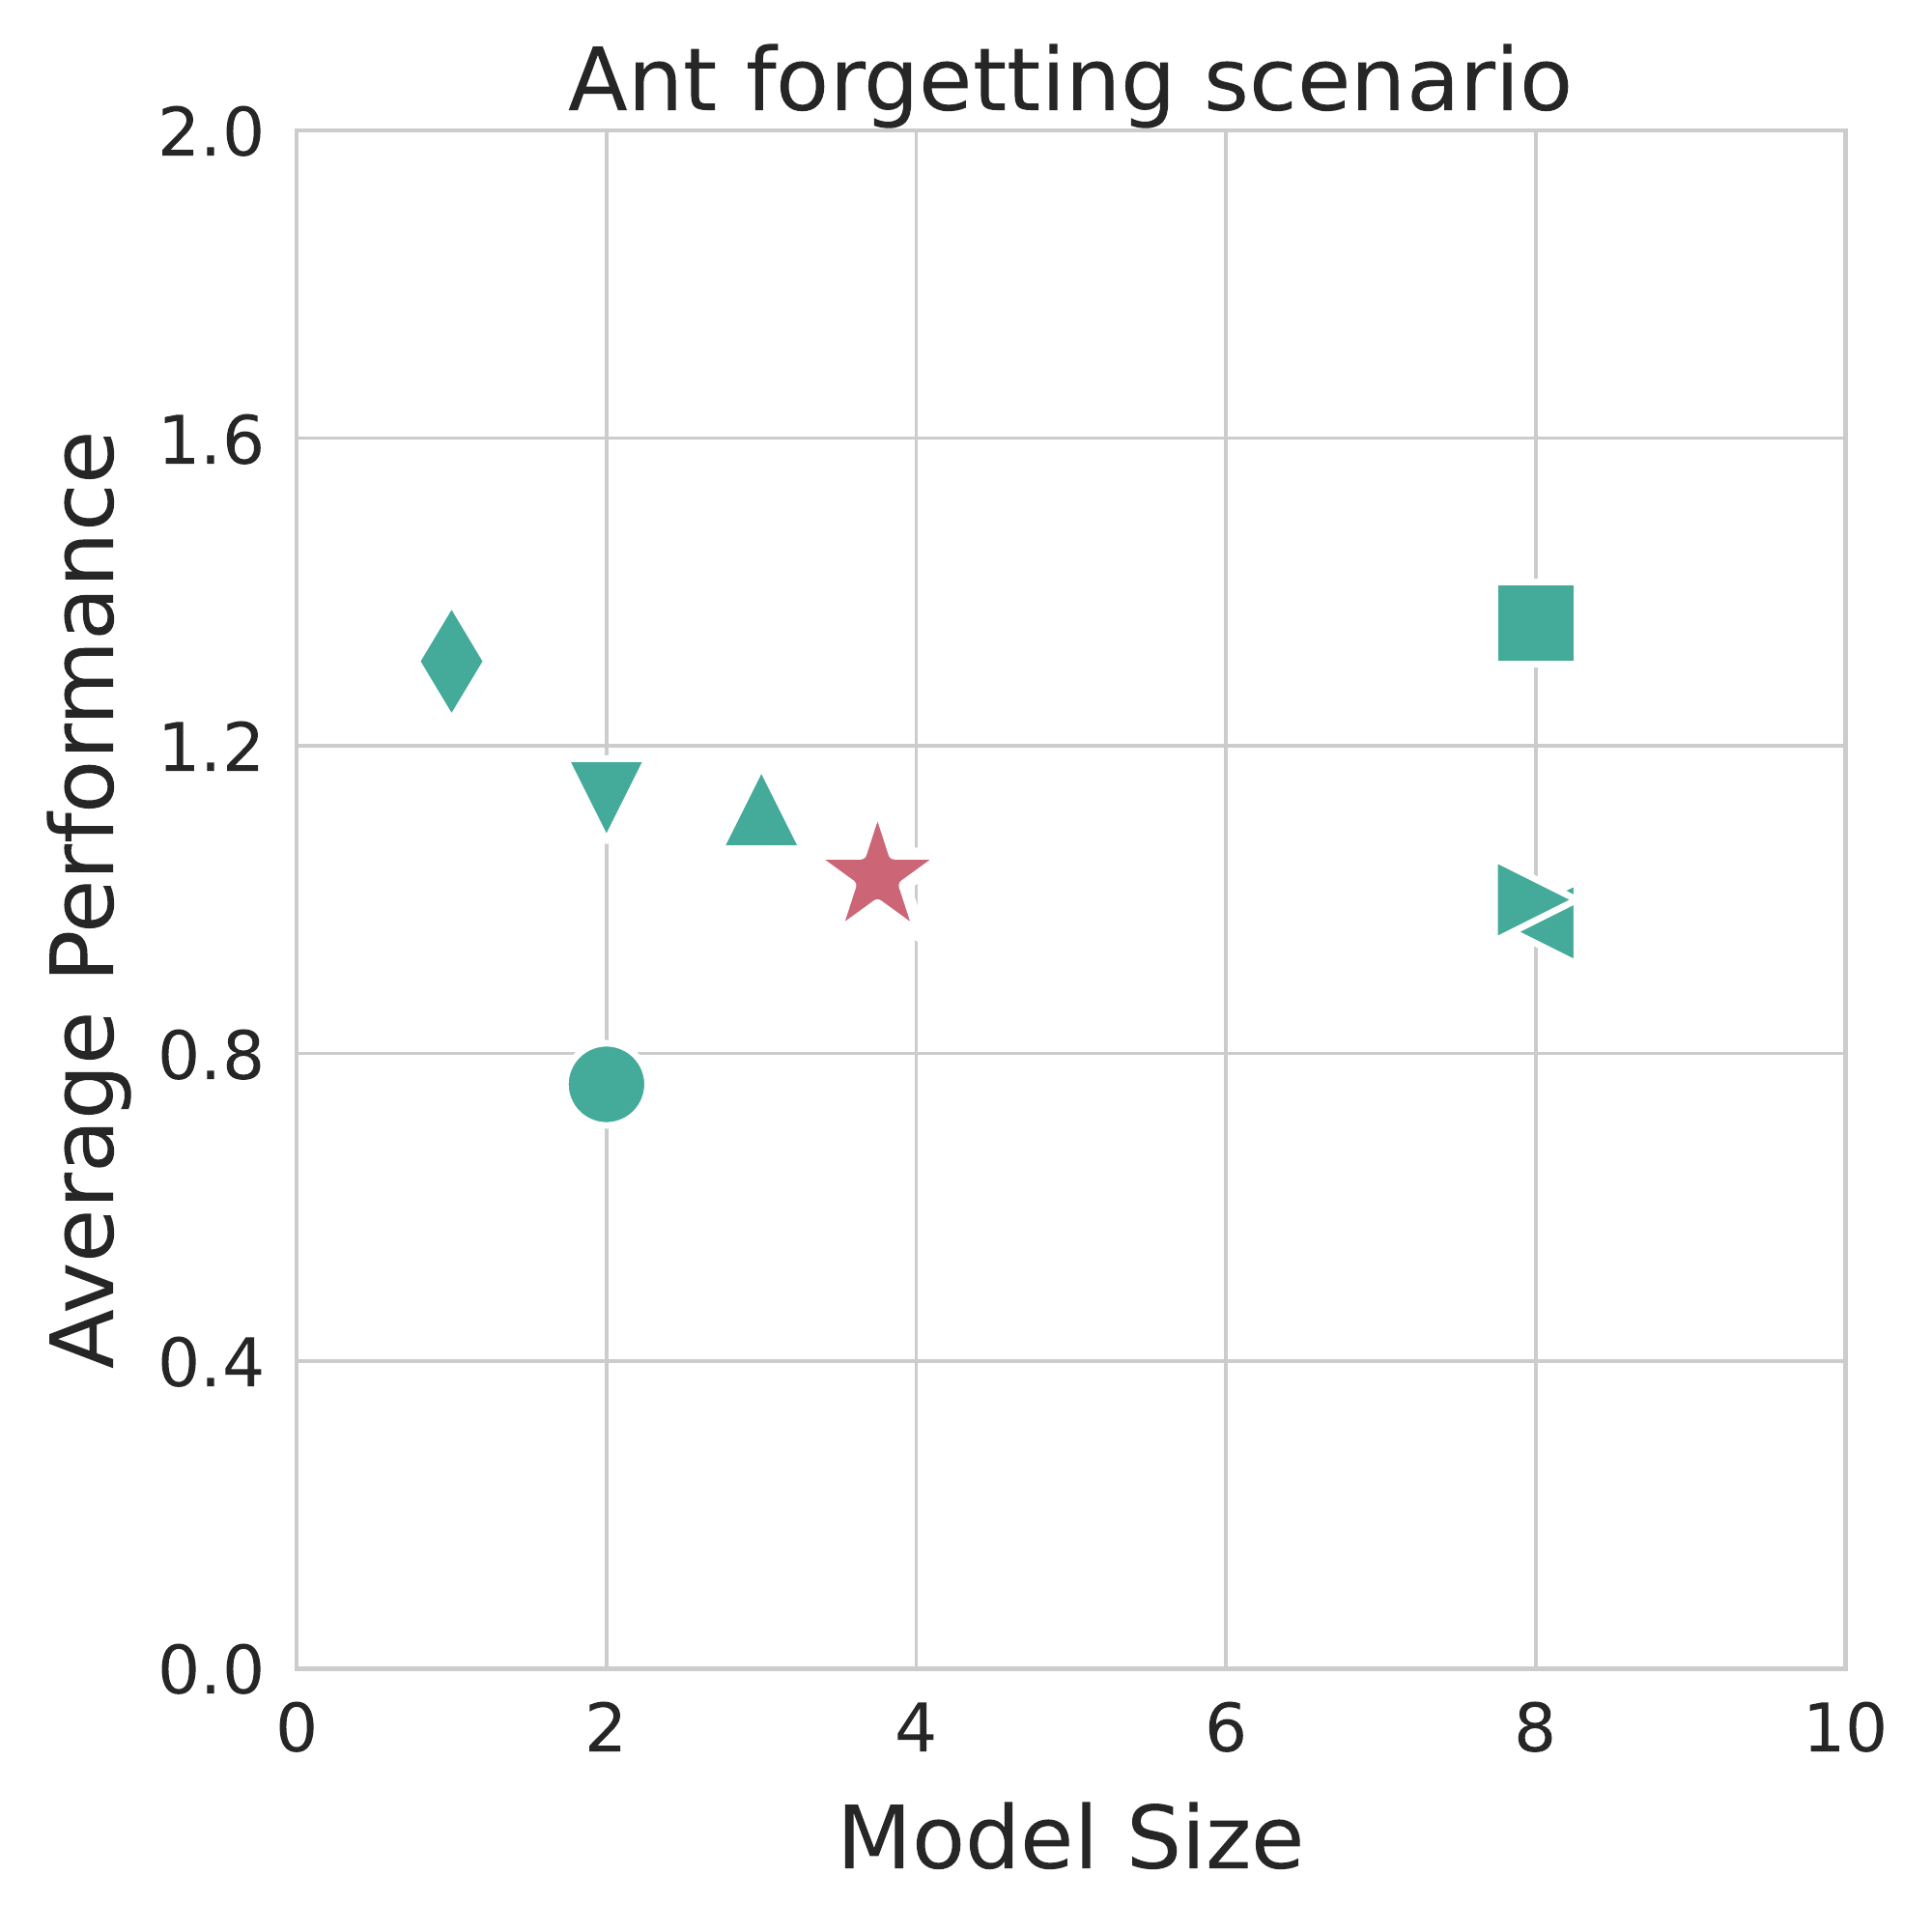}
     \end{subfigure}
     \hfill
     \begin{subfigure}[b]{0.4\textwidth}

        \includegraphics[width=\textwidth]{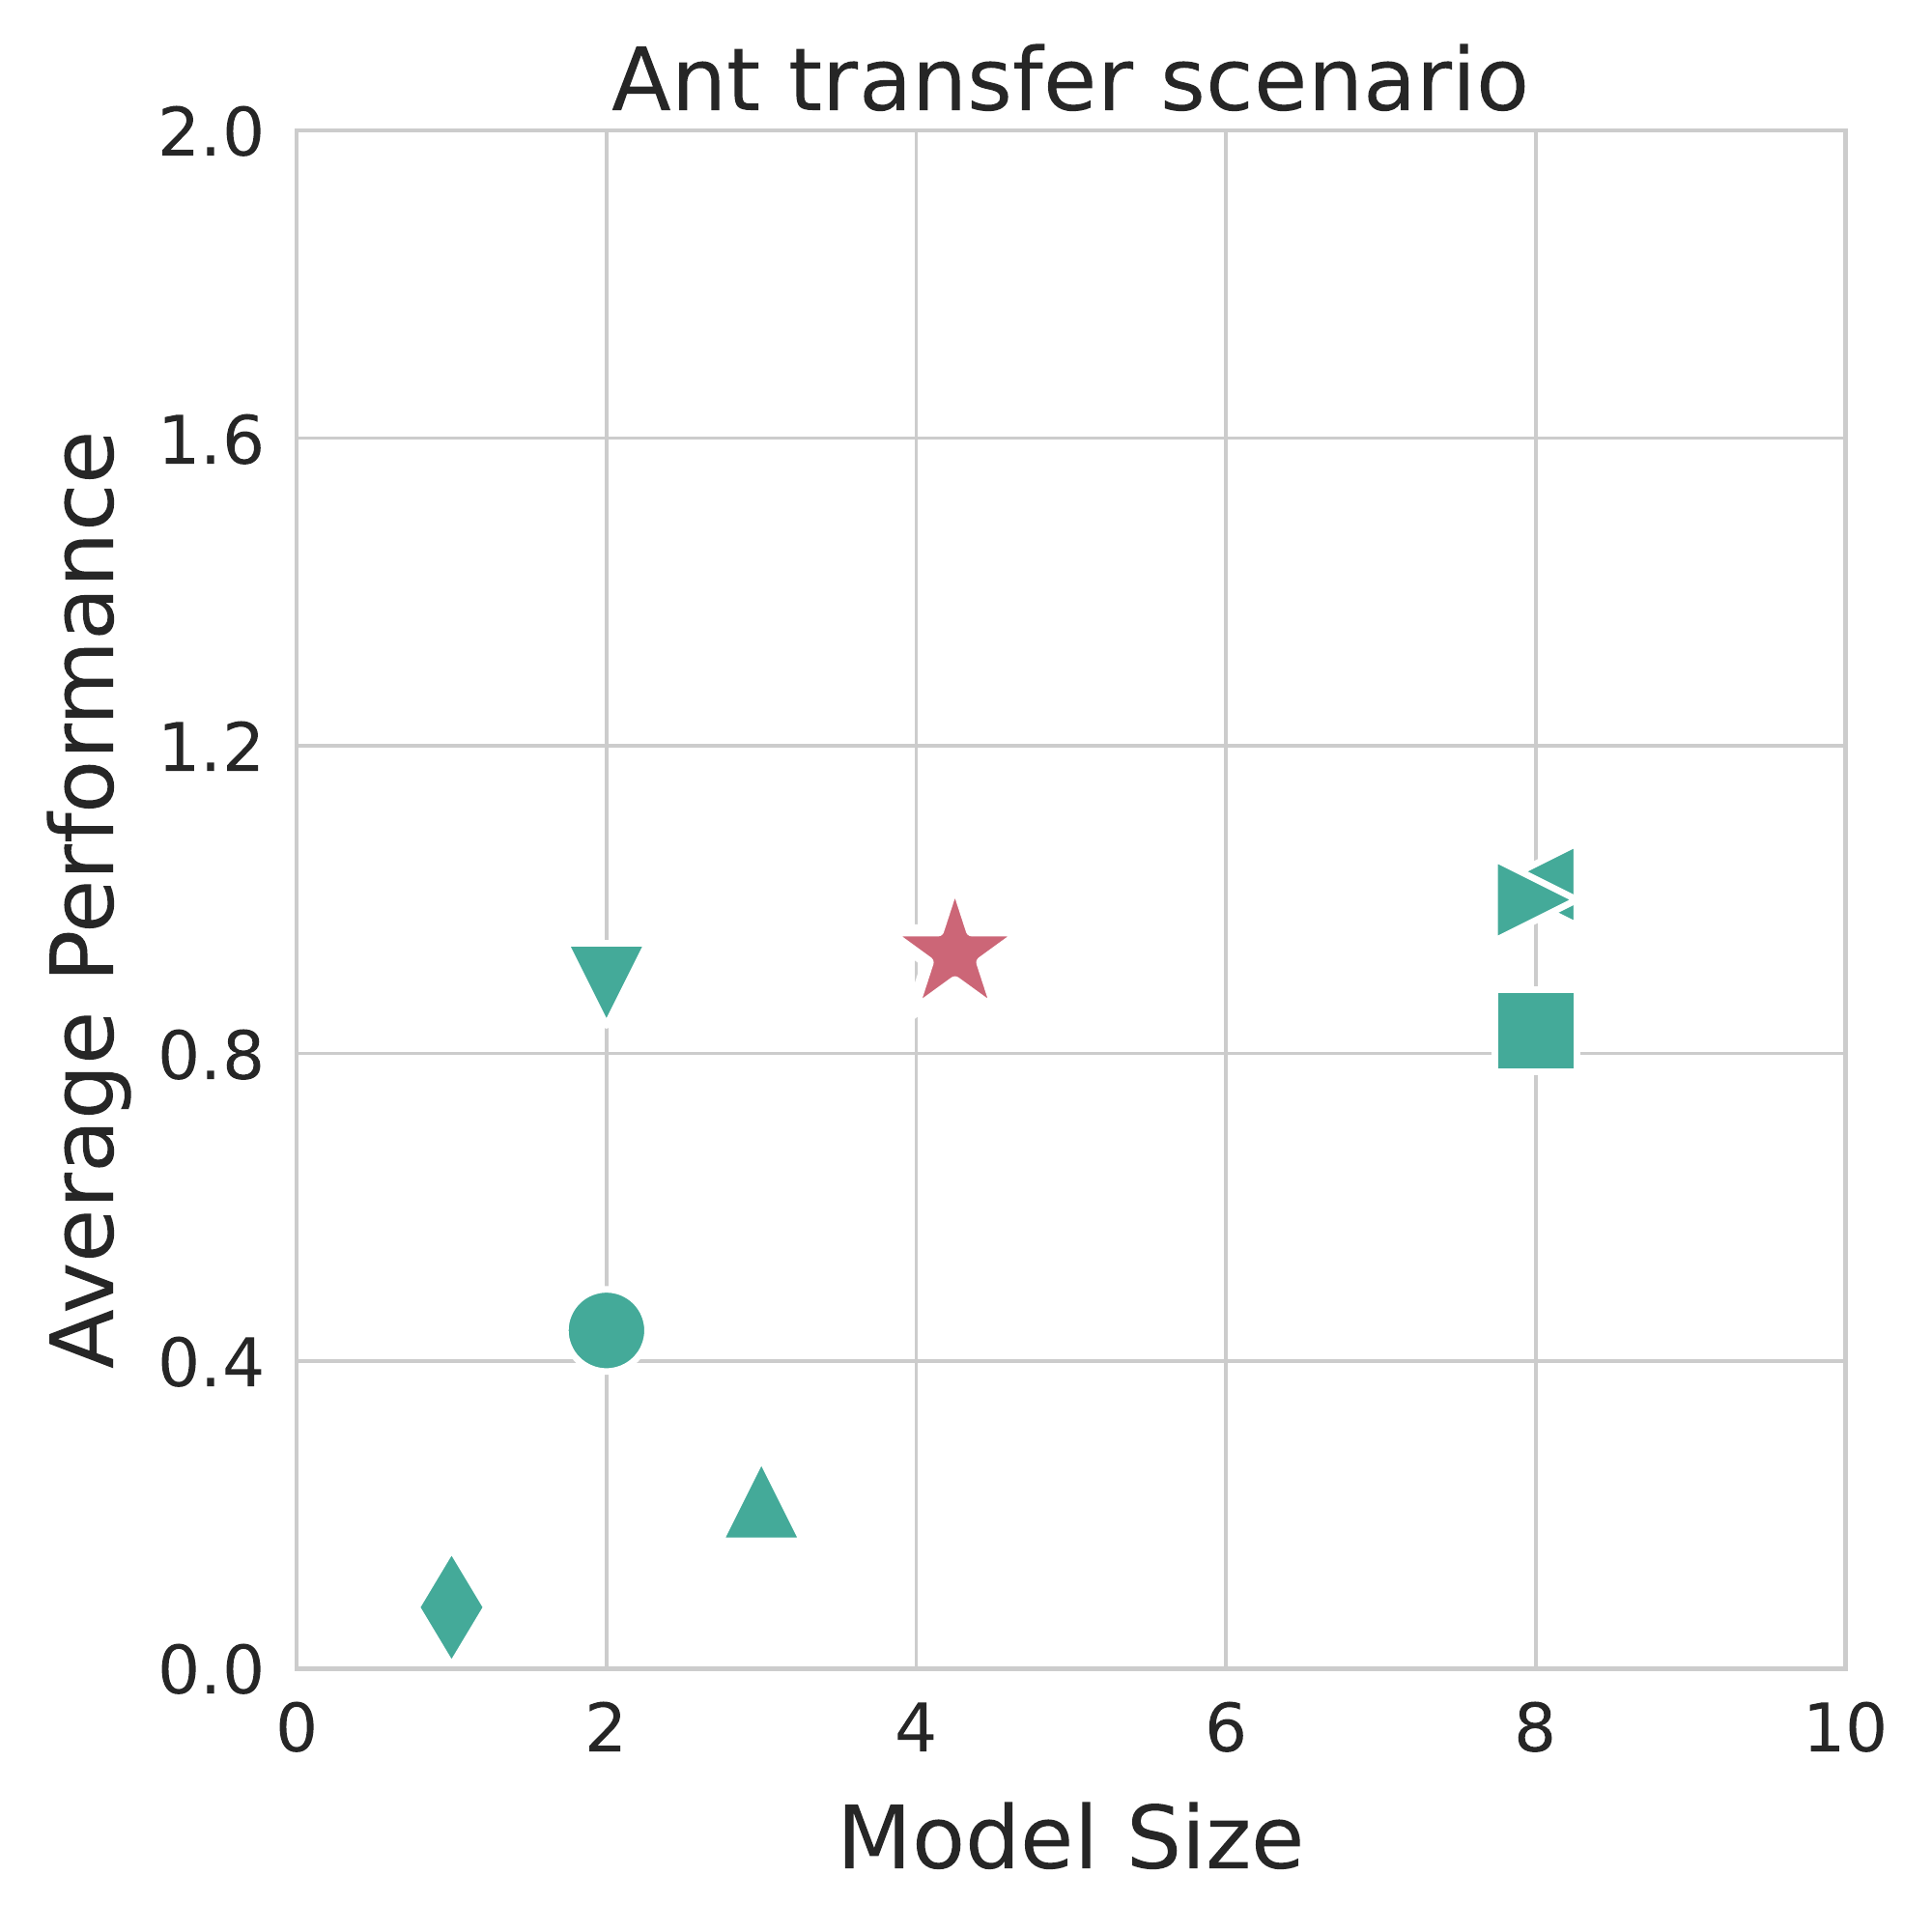}
     \end{subfigure}}
     \adjustbox{center}{
     \begin{subfigure}[b]{0.4\textwidth}

        \includegraphics[width=\textwidth]{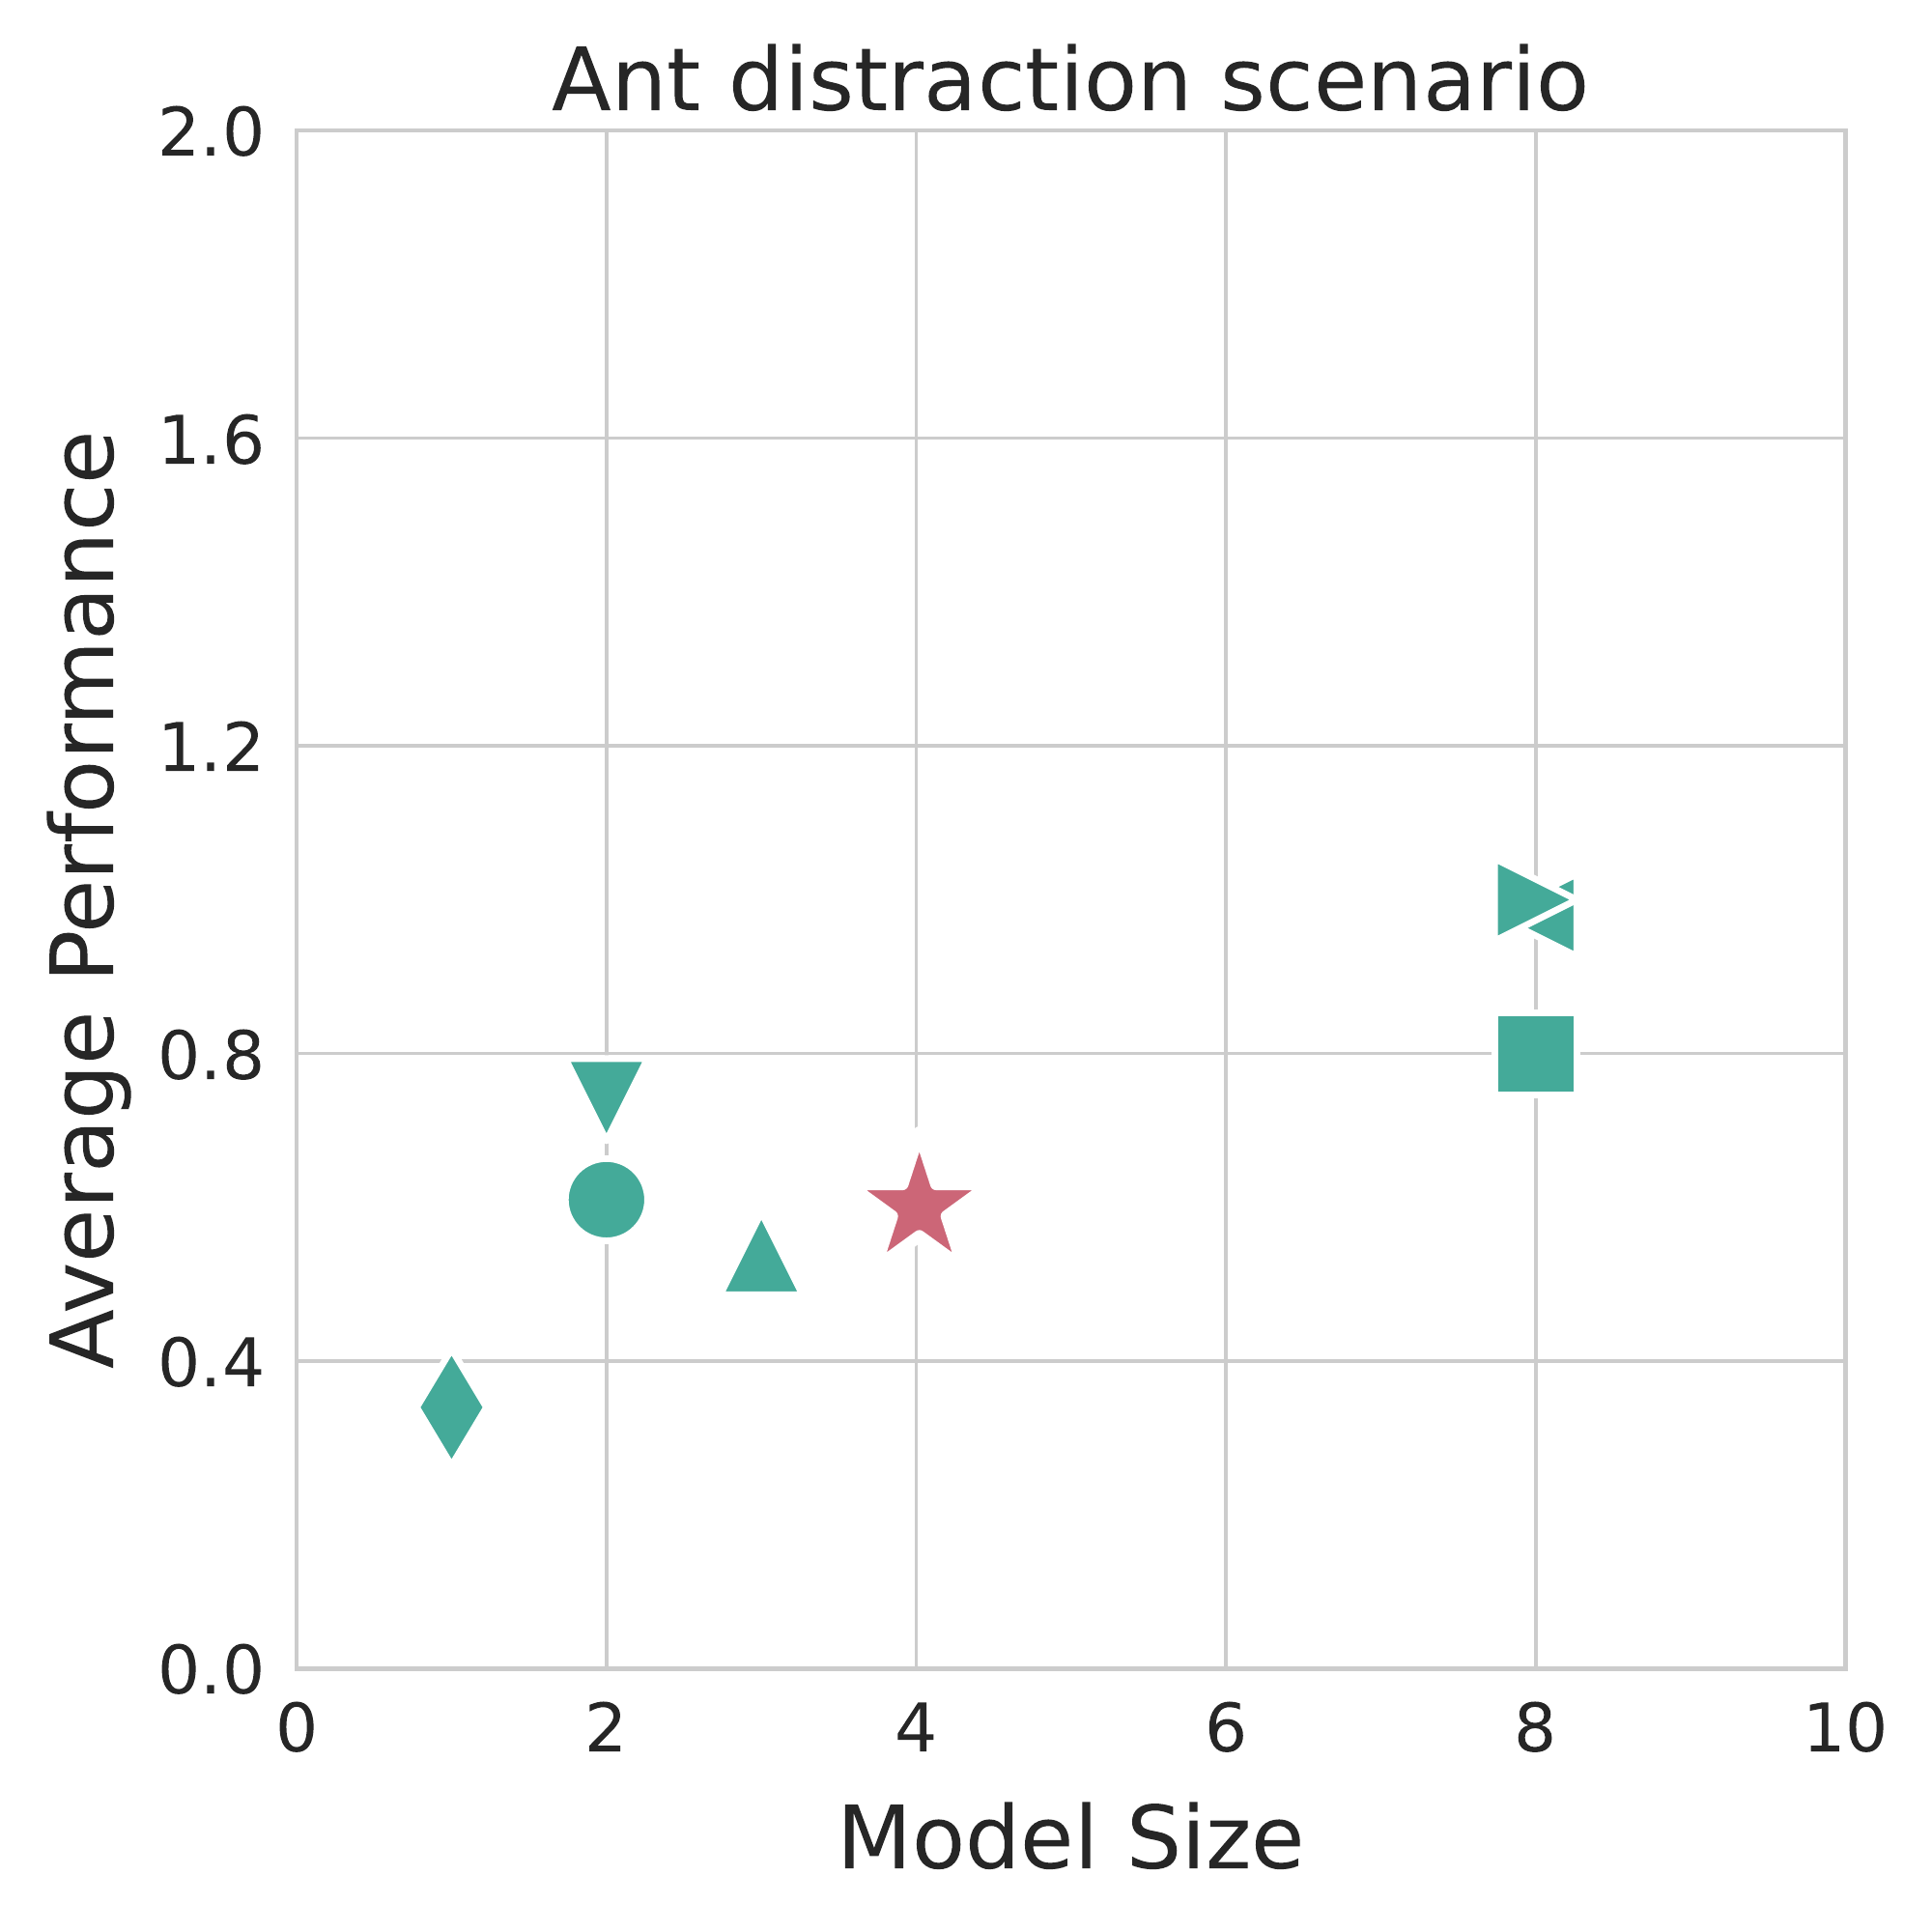}
     \end{subfigure}
     \hfill
     \begin{subfigure}[b]{0.4\textwidth}
        \includegraphics[width=\textwidth]{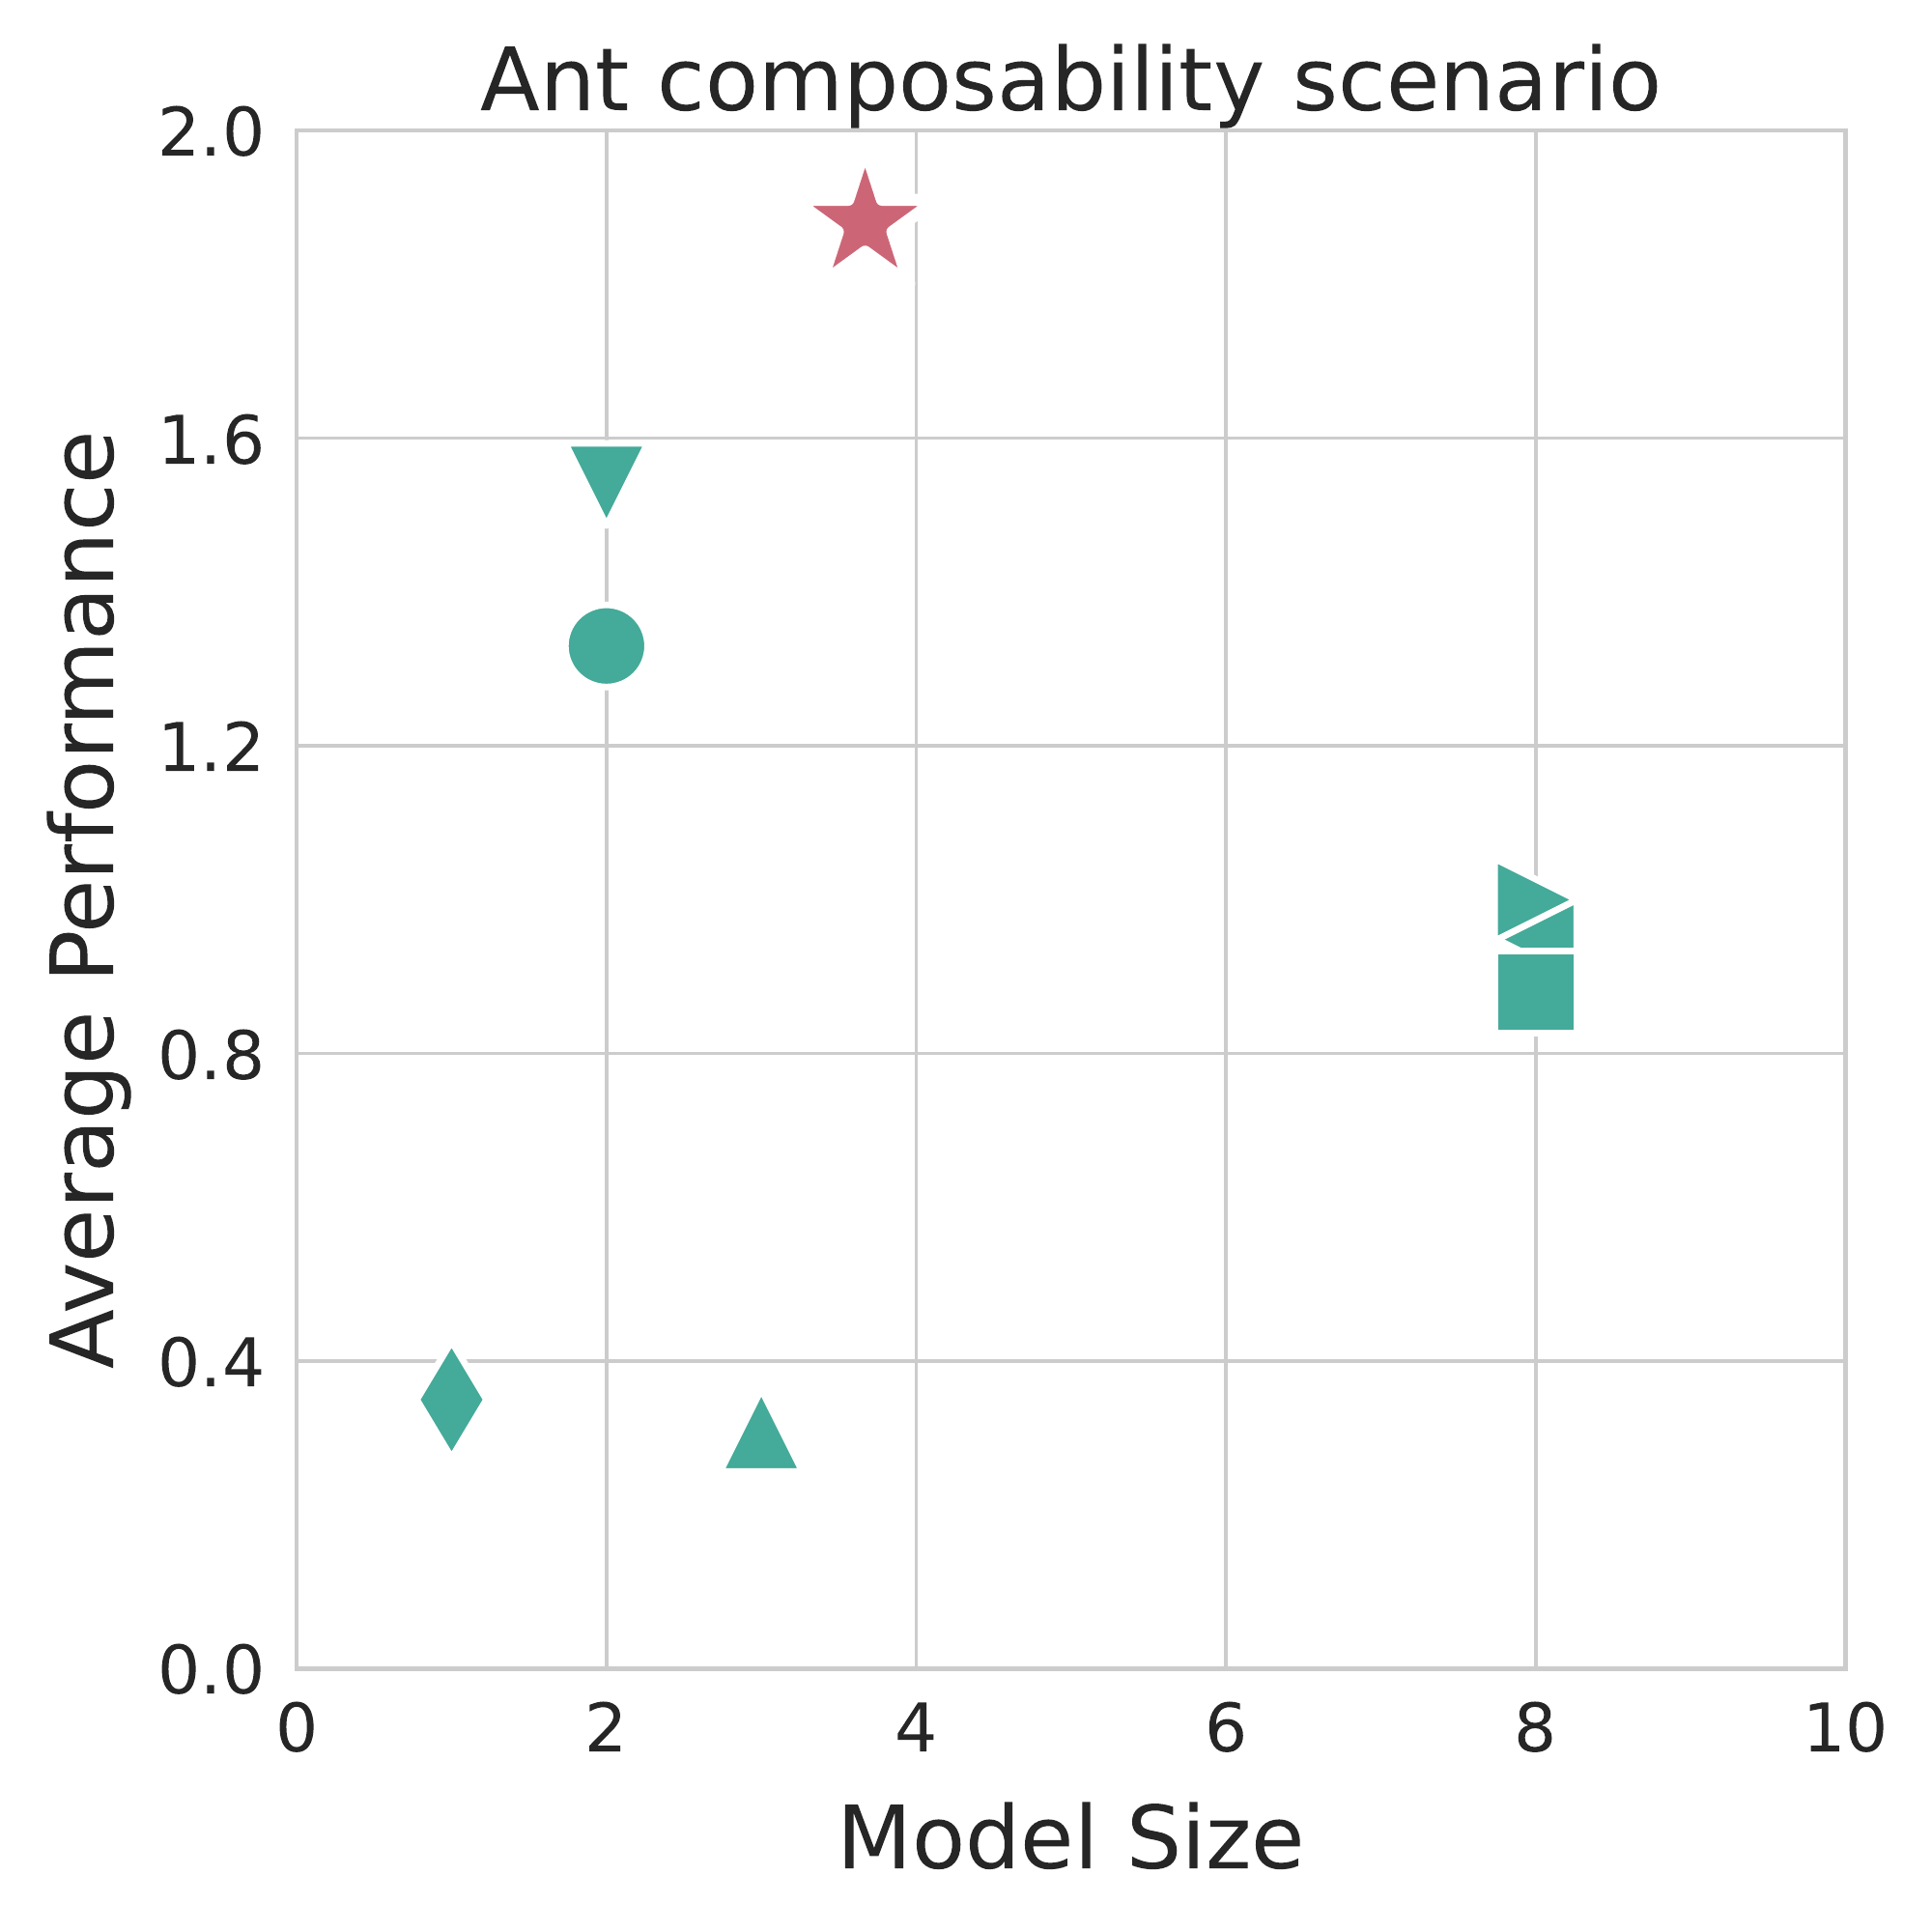}
     \end{subfigure}
     \hfill
     \begin{subfigure}[b]{0.4\textwidth}
        \includegraphics[width=\textwidth]{figures/ant_transfer_long_tradeoff.pdf}
     \end{subfigure}
     \\
     }
     \begin{subfigure}[b]{1.\textwidth}
         \centering
        \includegraphics[width=1.\textwidth]{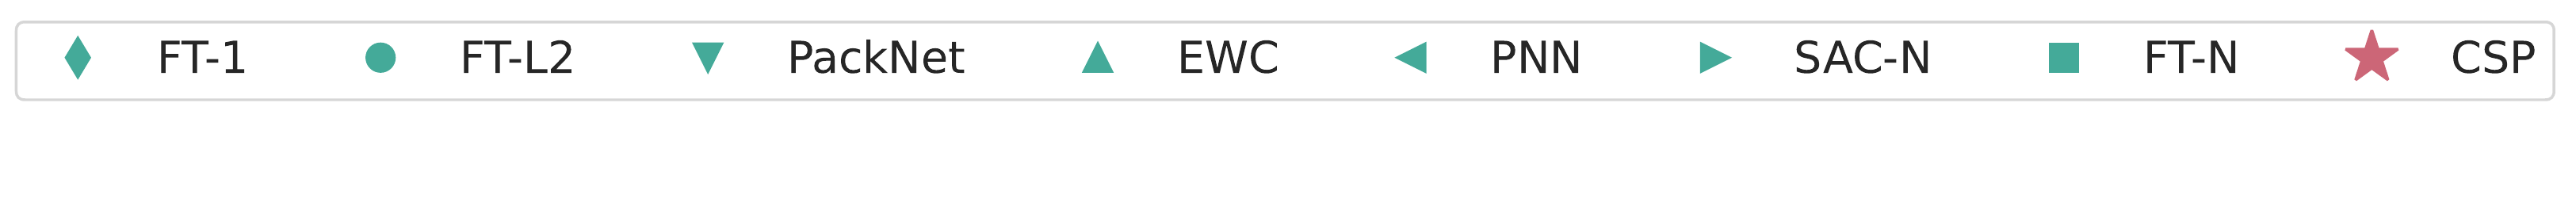}
     \end{subfigure}
    \caption{Performance-size trade-off for the 9 continuous control scenarios from Brax. Results are averaged over 10 seeds.}
    \label{fig:brax_detailed_tradeoff}
\end{figure}

\subsection{HalfCheetah}

For each of the 4 scenarios, we ran two versions: A short one (4 tasks) and a long one (8 tasks, the short one repeated twice). The normalized results are respectively presented in Table~\ref{tab:halfcheetah_4_tasks} and Table~\ref{tab:halfcheetah_8_tasks}. For a complete transparency, we also provide in Table~\ref{tab:halfcheetah_references} the raw rewards that were used to normalize the results. See Section \ref{app:exp} for more details about the computation of the normalized results. The best hyper-parameter sets for each scenario are provided in Table~\ref{tab:halfcheetah_hps}
\input{tables/halfcheetah_references}
\vspace{5mm}
\input{tables/halfcheetah_hps}
\input{tables/halfcheetah_8_tasks}

\newpage
\subsection{Ant}

We only ran the short version of the 4 scenarios. The long version is currently running and will be displayed in a future version of this paper. The normalized results are respectively presented in Table~\ref{tab:ant_4_tasks}. For a complete transparency, we also provide in Table~\ref{tab:ant_references} the raw rewards that were used to normalize the results. See Section \ref{app:exp} for more details about the computation of the normalized results. The best hyper-parameter sets for each scenario are provided in Table~\ref{tab:ant_hps}

\input{tables/ant_references}
\vspace{5mm}
\input{tables/ant_hps}
\newpage
\input{tables/ant_8_tasks}
\newpage
%\input{tables/ant_8_tasks}

\subsection{Continual World}
We provide the final average performance of the methods over the 8 triplets proposed in \cite{Woczyk2021ContinualWA}. See Table~\ref{cw_triplets}.

\vspace{15mm}

\input{tables/cw_triplets}

\newpage

\subsection{Humanoid}

We designed an additional short scenario on Humanoid and try our methods and baselines on it. 
\input{tables/humanoid_references}
\vspace{5mm}
\input{tables/humanoid_hps}
\input{tables/humanoid_4_tasks}
\newpage


\subsection{Additional ablation}

We ran additional experiments to verify the robustness of our model with respect to the diversity of the task sequence. To do so, we designed 3 different sequences with 10 tasks each on Halfcheetah. One with \textit{similar} tasks where each task in the sequence is selected to have the largest possible forward transfer from the previous task according to Figure~\ref{fig:forward_transfer}, one with \textit{dissimilar} tasks where each task in the sequence is selected to have the lowest possible forward transfer from the previous task according to Figure~\ref{fig:forward_transfer}, and one with \textit{random} tasks which are sampled uniformly from the entire set of tasks. Here are the sequences:

\newlist{sequences}{enumerate}{3}
\setlist[sequences]{label*=\arabic*.}
\setlistdepth{1}
\begin{sequences}
    \item \textbf{Similar:}\\\texttt{normal → hugefoot →carry\_stuff → defective\_module → tinyfoot\_moon → hugefoot\_rainfall → moon → tinyfoot → rainfall → carry\_stuff\_hugegravity} \\
    \item \textbf{Random:}\\ \texttt{tinyfoot → normal → hugefoot\_rainfall → moon → defective\_module → carry\_stuff\_hugegravity → rainfall → hugefoot → tinyfoot\_moon → carry\_stuff} \\
    \item \textbf{Dissimilar:}\\ \texttt{carry\_stuff\_hugegravity → moon → defective\_module → hugefoot\_rainfall → normal → tinyfoot → hugefoot → carry\_stuff → tinyfoot\_moon → rainfall} \\
\end{sequences}

We report the growing factor with respect to the threshold (see Figure~\ref{fig:ablation_tasks}). Our results indicate that the diversity of the tasks doesn't have a significant impact on the final size of our model. Thus, our method is robust to the degree of transfer across tasks, demonstrating that it can handle just as well sequences of tasks with large negative transfer among them. As expected, the growing factor decreases as the threshold increases. Hence, the threshold can be used to control how much the size of the model grows with the number of tasks, allowing CSP to scale to long task sequences without prohibitive memory and computational requirements. 

\input{}

\begin{figure}[t!]
    \centering
    \includegraphics[width=0.8\linewidth]{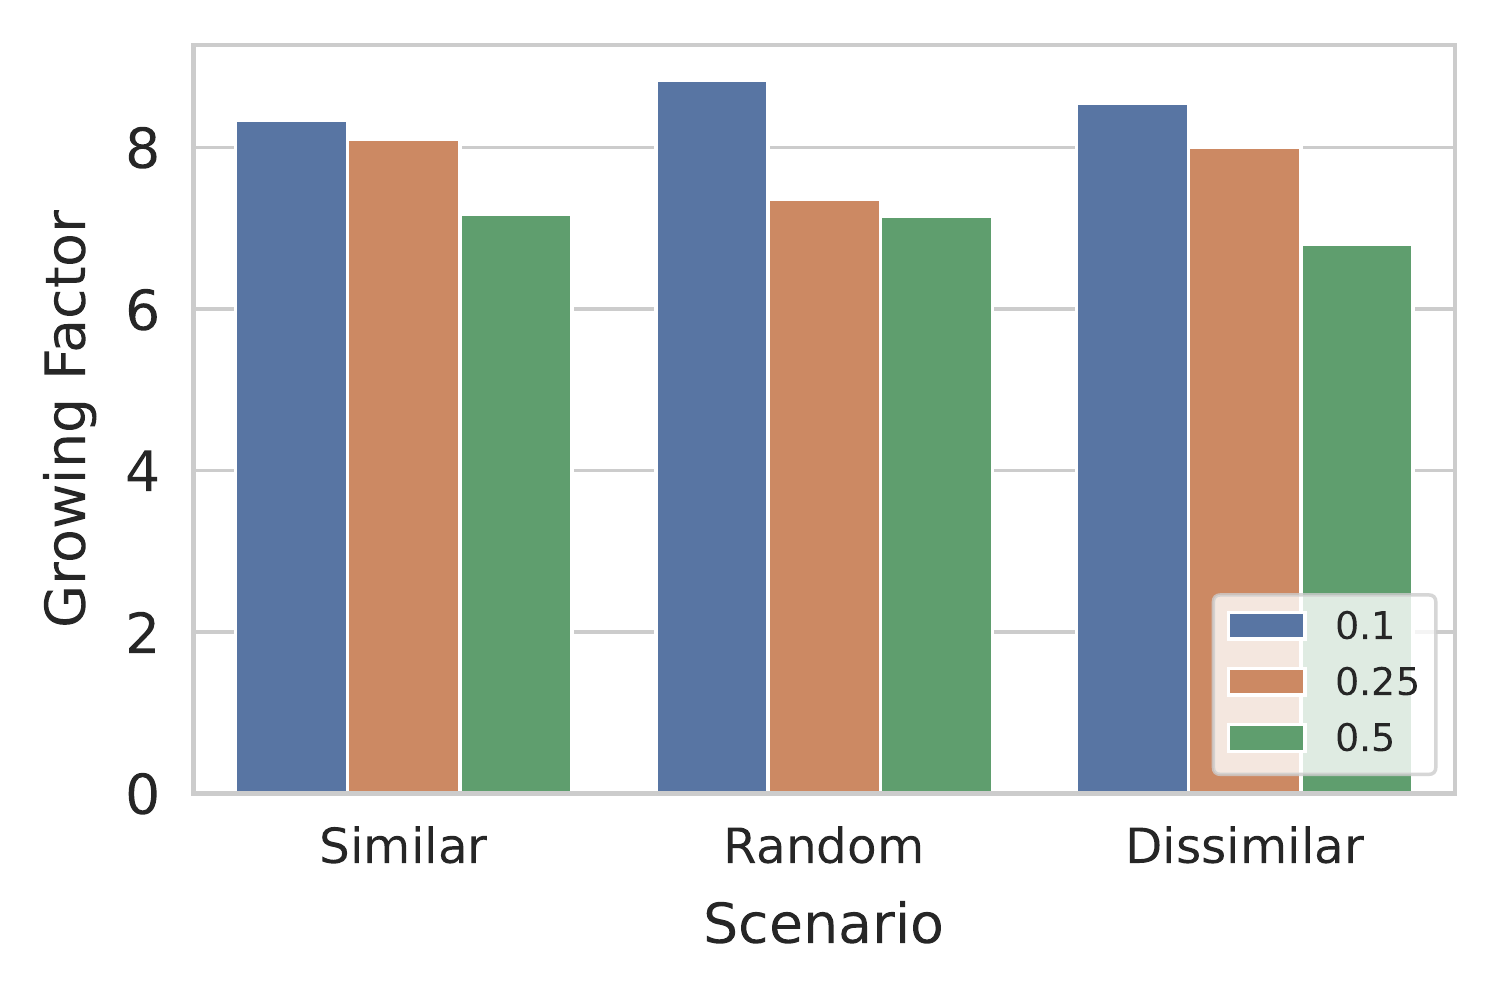}
    \caption{Growing factor evolution of our model CSP in different scenario with different thresholds.}
    \label{fig:ablation_tasks}
\end{figure}
